# Supplementary material for: A theory of quantum subspace diagonalization
Source: arXiv:2110.07492 source file (2023-06-13)
Supplement: Supplementary file 1 [file revision1_supplement.tex]

% SIAM Supplemental File Template
\documentclass[review,supplement,onefignum,onetabnum]{siamart190516}

\input{ex_shared}
\usepackage{amsmath}

\externaldocument{revision1}

\headers{A Theory of QSD}{E. N. Epperly, L. Lin, and Y. Nakatsukasa}

% Optional PDF information
\ifpdf
\hypersetup{
  pdftitle={Supplementary Materials: A Theory of Quantum Subspace Diagonalization},
  pdfauthor={E. N. Epperly, L. Lin, and Y. Nakatsukasa}
}
\fi

\begin{document}

\maketitle

In this supplement, we provide additional proofs and numerical experiments to support the claims made in the main text.

\input{supplement_core.tex}

\bibliographystyle{siamplain}
\bibliography{references}

\end{document}
